# Supplementary material for: Cell Detection by Functional Inverse Diffusion and Non-negative Group Sparsity$-$Part II: Proximal Optimization and Performance Evaluation
Source: arXiv:1710.01622 ancillary file (2018-10-17)
Supplement: Supplementary file 1 [file supp_mat.pdf]

# Cell Detection by Functional Inverse Diffusion and Group Sparsity - Supplementary Material

Pol del Aguila Pla* and Joakim Jaldén
*poldap@kth.se, https://people.kth.se/~poldap/

**Abstract**

Throughout our two-part paper, we often encounter derivations that are quite straight-forward, but are still lengthy and challenging to obtain. Here, we include those derivations and content that are not novel or relevant enough to be included in the paper but may help the interested reader and provide more detail on some of our arguments. Finally, we also include some additional experimental results and material to help in reproducing our results.

In this document, then, we will provide detail on each point that we deem will benefit from it, in the order these points arise in our two-part paper.

## CONTENTS

**I Part I – Modeling and Inverse Problems** 2
- I-A Convolving the Green function with the SDR . . . 2
- I-B Simulating data from our physical model . . . 2
- I-C Discretization results . . . 4

**II Part II – Proximal Optimization and Performance Evaluation** 6
- II-A Proximal operator of the non-negative weighted norm in $\mathcal{X}$ . . . 6
- II-B More on kernels and their approximation . . . 6
- II-C Experimental results . . . 7

**References** 7

# I. Part I – Modeling and Inverse Problems

## A. Convolving the Green function with the SDR

Between [1, Section II, Equations (3) and (4)], there is a rather long step. Recall here that

$$p(\mathbf{r},t) = \int_0^t g_{\sqrt{2D\tau}}(\mathbf{r})\varphi(\tau,t)\mathrm{d}\tau\,.$$

Then, [1, Equation (3)] states that

$$d(\mathbf{r},t) = (s * p)(\mathbf{r},t)\,. \tag{1}$$

Consider the following derivation

$$\begin{aligned}
d(\mathbf{r},t) &= \int_{\mathbb{R}^2}\int_0^t s(\boldsymbol{\rho},\omega)p(\mathbf{r}-\boldsymbol{\rho},t-\omega)\mathrm{d}\omega\mathrm{d}\boldsymbol{\rho}\\
&= \int_{\mathbb{R}^2}\int_0^t\int_0^{t-\omega} s(\boldsymbol{\rho},\omega)g_{\sqrt{2D\tau}}(\mathbf{r}-\boldsymbol{\rho})\varphi(\tau,t-\omega)\mathrm{d}\tau\mathrm{d}\omega\mathrm{d}\boldsymbol{\rho}\\
&\overset{(!)}{=} \int_{\mathbb{R}^2}\int_0^t\int_0^{t-\tau} s(\boldsymbol{\rho},\omega)g_{\sqrt{2D\tau}}(\mathbf{r}-\boldsymbol{\rho})\varphi(\tau,t-\omega)\mathrm{d}\omega\mathrm{d}\tau\mathrm{d}\boldsymbol{\rho}\\
&= \int_{\mathbb{R}^2}\int_0^t g_{\sqrt{2D\tau}}(\mathbf{r}-\boldsymbol{\rho})\int_0^{t-\tau} s(\boldsymbol{\rho},\omega)\varphi(\tau,t-\omega)\mathrm{d}\omega\mathrm{d}\tau\mathrm{d}\boldsymbol{\rho}\\
&\overset{(!!)}{=} \int_0^t\int_{\mathbb{R}^2} g_{\sqrt{2D\tau}}(\mathbf{r}-\boldsymbol{\rho})\int_\tau^t s(\boldsymbol{\rho},t-\eta)\varphi(\tau,\eta)\mathrm{d}\eta\mathrm{d}\boldsymbol{\rho}\mathrm{d}\tau\\
&= \int_0^t\int_{\mathbb{R}^2} g_{\sqrt{2D\tau}}(\mathbf{r}-\boldsymbol{\rho})v(\boldsymbol{\rho},\tau,t)\mathrm{d}\boldsymbol{\rho}\mathrm{d}\tau\\
&= \int_0^t G_{\sqrt{2D\tau}}v(\mathbf{r},\tau,t)\mathrm{d}\tau \qquad (2)\\
&= \int_0^{\sigma_{\max}} G_\sigma a_\sigma \mathrm{d}\sigma\,. \qquad (3)
\end{aligned}$$

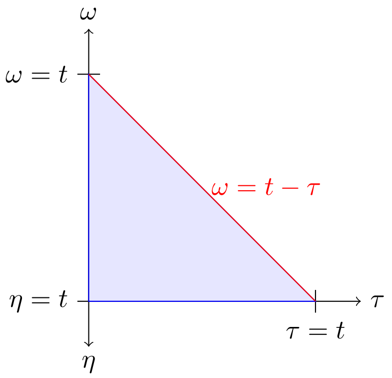


Three equivalent representations of the area in the drawing, all used in the derivation of the main formula for $d(\mathbf{r},t)$ in (2). Note here that $\eta = t-\omega$.

Note that $v$ is defined in [1, Equation (5)] as

$$v : \mathbb{R}^2 \times \mathbb{R}_+^2 \to \mathbb{R}_+ \text{ such that } v(\mathbf{r},\tau,t) = \int_\tau^t s(\mathbf{r},t-\eta)\varphi(\tau,\eta)\mathrm{d}\eta\,,$$

and (2) is precisely [1, Equation (4)]. The changes of integration margins (!) and variables (!!) are based on the interpretation of the integration region in the figure to the right, which basically gives that the integration region can be described as

$$\{(\omega,\tau) : \omega\in[0,t] \text{ and } \tau\in[0,t-\omega]\}\,,\ \text{or, } \{(\omega,\tau) : \tau\in[0,t] \text{ and } \omega\in[0,t-\tau]\}\,,\ \text{or } \{(\eta,\tau) : \tau\in[0,t] \text{ and } \eta\in[\tau,t]\}\,,$$

with $\eta = t-\omega$. Finally, the step from (2) to (3) is simply the change of variables $\sigma = \sqrt{2D\tau}$, which is what takes us to the definition of $a : \Omega \to \mathbb{R}_+$ as in [1, Equation (7)].

## B. Simulating data from our physical model

In [1] we give a detailed expression for $\varphi$ with respect to $\kappa_\mathrm{a}$, $\kappa_\mathrm{d}$ and $D$, in terms of an infinite sum. Recall here that that expression was

$$\varphi(\tau,t) = i_{[0,t)}(\tau)\sum_{j=1}^{\infty}\phi^{j*}(\tau)p\left[j-1;\kappa_\mathrm{d}(t-\tau)\right]\,, \tag{4}$$

where $\phi^{j*}$ was the $j$-th convolutional power of $\phi$ and $p[j;\lambda]$ was the Poisson probability mass function with parameter $\lambda$ evaluated at $j$. There, we also proved that truncating the sum can result in an arbitrarily small error for any valid $(\tau,t)$ (see [1] for details). Nonetheless, obtaining simulated data from our model from these results is not trivial.

The fundamental steps to follow are clear. First, one has to draw a random SDR $s$ according to a certain design. Second, one has to obtain the corresponding PSDR $a$. Finally, one can use the discretized operator in [1] to obtain a simulated image. Of these three steps, the first and the last are basic and deserve no attention here, but the second can be challenging.

Recall first the expression for $v$ at the observation time $T$ from [1]

$$v(\mathbf{r},\tau,T) = \int_\tau^T s(\mathbf{r},T-\eta)\varphi(\tau,\eta)\mathrm{d}\eta\,, \tag{5}$$

and recall that $v$ at time $T$ is a complete parallel to the PSDR $a$ in which the free time in diffusion is still expressed as a time variable, instead of expressing it with respect to the corresponding kernel width $\sigma$ (as in the PSDR). In other words, $v$ at the observation time $T$ represents the density of particles released from $\mathbf{r}$ that are found in the final image after having been in Brownian motion for a period of $\tau$ seconds.

We will first focus on how, given a discrete SDR at a certain location $\mathbf{r}$ (i.e., for one particular cell), one can compute values of $v$ at time $T$, i.e, $v(\mathbf{r},\tau,T)$ for specific $\tau$s. Consider then a discrete SDR at a certain position $\mathbf{r}$, i.e., $s_{\mathbf{r}}$, with respect to the inner approximation paradigm, i.e. a piece-wise constant function $s_{\mathbf{r}}$ such that

$$s_{\mathbf{r}}(t)=\sum_{n=1}^{N_t}\tilde{s}_{\mathbf{r}}[n]i_{[(n-1)\Delta_t,n\Delta_t]}(t)\,,$$

where $N_t$ is, as in [2], the number of discretization points in time, and $\Delta_t=T/N_t$, while $n$ is just a discrete variable with no relation to the $n$ used to discretize the spatial dimension $x$. Consider now a specific time in free motion $\tau$ such that $\tau=n_\tau\Delta_t$, for some $n_\tau\in\{1,2,\dots,N_t\}$. Then, we have that

$$\begin{aligned}
v(\mathbf{r},\tau,T)&=\int_\tau^T s_{\mathbf{r}}(T-\eta)\varphi(\tau,\eta)\mathrm{d}\eta=\sum_{j=1}^{\infty}\phi^{j*}(\tau)\int_\tau^T s_{\mathbf{r}}(T-\eta)p[j-1;\kappa_{\mathrm{d}}(\eta-\tau)]i_{[0,\eta)}(\tau)\mathrm{d}\eta\\
&=\sum_{j=1}^{\infty}\phi^{j*}(\tau)\int_\tau^T s_{\mathbf{r}}(T-\eta)p[j-1;\kappa_{\mathrm{d}}(\eta-\tau)]\mathrm{d}\eta\\
&=\sum_{j=1}^{\infty}\phi^{j*}(\tau)\sum_{n=1}^{N_t}\tilde{s}_{\mathbf{r}}[n]\int_\tau^T i_{[(n-1)\Delta_t,n\Delta_t]}(T-\eta)p[j-1;\kappa_{\mathrm{d}}(\eta-\tau)]\mathrm{d}\eta\\
&=\sum_{j=1}^{\infty}\phi^{j*}(\tau)\sum_{n=1}^{N_t-n_\tau}\tilde{s}_{\mathbf{r}}[n]\int_\tau^T i_{[(N_t-n)\Delta_t,(N_t-n+1)\Delta_t]}(\eta)p[j-1;\kappa_{\mathrm{d}}(\eta-\tau)]\mathrm{d}\eta\\
&=\sum_{j=1}^{\infty}\phi^{j*}(\tau)\sum_{n=1}^{N_t-n_\tau}\tilde{s}_{\mathbf{r}}[n]\int_{(N_t-n)\Delta_t}^{(N_t-n+1)\Delta_t} p[j-1;\kappa_{\mathrm{d}}(\eta-\tau)]\mathrm{d}\eta\\
&\approx\Delta_t\sum_{j=1}^{\infty}\phi^{j*}(\tau)\sum_{n=1}^{N_t-n_\tau}\tilde{s}_{\mathbf{r}}[n]\;p[j-1;\kappa_{\mathrm{d}}(T-\tau-\Delta_t(n+1/2))]\,.
\end{aligned}$$

This expression, then, allows us to build an approximation of the density $v(\mathbf{r},\tau,T)$ at this specific position $\mathbf{r}$ as a function of $\tau$ that will be more precise around values of $\tau$ multiple of $\Delta_t$, i.e.,

$$\tilde{v}_{\mathbf{r}}(\tau)=\sum_{m=1}^{N_t}\left(\Delta_t\sum_{j=1}^{\infty}\phi^{j*}(\tau)\sum_{n=1}^{N_t-m}\tilde{s}_{\mathbf{r}}[n]\;p[j-1;\kappa_{\mathrm{d}}(T-\tau-\Delta_t(n+1/2))]\right)i_{[(m-1)\Delta_t,m\Delta_t]}(\tau)\,.$$

This approximation simplifies the progressive restriction of the integration range in (5) with an artificial step behavior in the inner sum. Note that this approximation can be improved by increasing the number of time-points $N_t$ in the simulation for the same total time $T$.

Our objective, however, is to obtain a piece-wise constant representation of the density $a_{\mathbf{r}}$ as a function in $\sigma$, so that we can use the expression of the discretized operator to obtain a simulated image (see [1]). To do so, we decide on a approximately regular grid in $\sigma$ such that each of the boundaries $\{\sigma_0,\sigma_1,\sigma_2,\dots,\sigma_{K_{\mathrm{g}}}\}$ fulfill that $\sigma_k=\sqrt{2D\Delta_t n_k}$ for some $n_k\in\{0,1,2,\dots,N_t\}$. Then, we use that $\int_{\sigma_{k-1}}^{\sigma_k}a_{\mathbf{r}}(\sigma)\mathrm{d}\sigma=\int_{\Delta_t n_{k-1}}^{\Delta_t n_k}v(\mathbf{r},\tau,T)\mathrm{d}\tau$ by considering the coefficients $\tilde{a}_{\mathbf{r}}[k]$ such that

$$\begin{aligned}
\tilde{a}_{\mathbf{r}}[k]&=\int_{\Delta_t n_{k-1}}^{\Delta_t n_k}\tilde{v}_{\mathbf{r}}(\tau)\mathrm{d}\tau=\Delta_t\sum_{j=1}^{\infty}\sum_{m=1}^{N_t}\sum_{n=1}^{N_t-m}\tilde{s}_{\mathbf{r}}[n]\int_{\Delta_t n_{k-1}}^{\Delta_t n_k}\phi^{j*}(\tau)\;p[j-1;\kappa_{\mathrm{d}}(T-\tau-\Delta_t(n+1/2))]i_{[(m-1)\Delta_t,m\Delta_t]}(\tau)\mathrm{d}\tau\\
&=\Delta_t\sum_{j=1}^{\infty}\sum_{m=n_{k-1}+1}^{n_k}\sum_{n=1}^{N_t-m}\tilde{s}_{\mathbf{r}}[n]\int_{(m-1)\Delta_t}^{m\Delta_t}\phi^{j*}(\tau)\;p[j-1;\kappa_{\mathrm{d}}(T-\tau-\Delta_t(n+1/2))]\mathrm{d}\tau &&(6)\\
&\approx\Delta_t\sum_{j=1}^{\infty}\sum_{m=n_{k-1}+1}^{n_k}\sum_{n=1}^{N_t-m}\tilde{s}_{\mathbf{r}}[n]p[j-1;\kappa_{\mathrm{d}}(T-\Delta_t(m+n))]\int_{(m-1)\Delta_t}^{m\Delta_t}\phi^{j*}(\tau)\mathrm{d}\tau &&(7)
\end{aligned}$$

and using them as parameters for a piece-wise constant approximation of the PSDR $\tilde{a}_{\mathbf{r}}(\sigma)$ as

$$\tilde{a}_{\mathbf{r}}(\sigma)=\sum_{k=1}^{K_{\mathrm{g}}}\frac{\tilde{a}_{\mathbf{r}}[k]}{\Delta_k}i_{[\sigma_{k-1},\sigma_k]}(\sigma)\,. \tag{8}$$

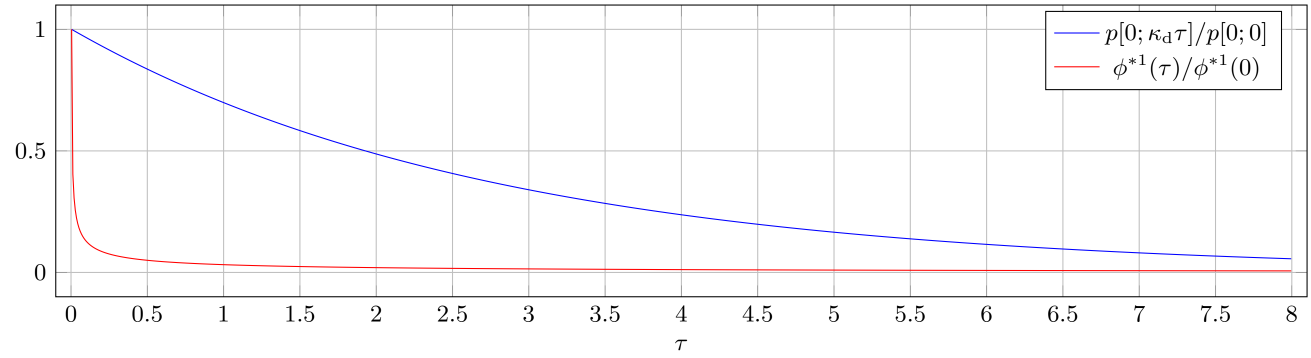


Fig. 1. Illustrative example. $p[j-1;\kappa_\mathrm{d}\tau]$ is smoother than $\phi^{*j}(\tau)$ for small $j$s. Illustration for $j=1$, $\kappa_\mathrm{d}=10^{-4}$ and $T=8$ h.

Intuitively, this piece-wise constant approximation is the result of simply obtaining the accumulated density in a region by using a related density, and then dividing that value by the lenght of the considered interval to estimate the desired density.

The approximation of the integral in going from (6) to (7) basically assumes that $p[\cdot,\cdot]$ is constant in an interval $\Delta_t$, or at least compared to $\phi^{j*}(\tau)$. This is specially true for low $j$s, from which most of the weight in the infinite sum comes. See, in particular, the case of $j=1$ in Figure 1, which shows the normalized dependence of both factors on $\tau$. Finally, to obtain $\int_{(m-1)\Delta_t}^{m\Delta_t}\phi^{j*}(\tau)\mathrm{d}\tau$ as in (7), one can initially compute the discrete approximation to the first $\phi^{1*}(\tau)$ by computation of this integral, and approximate the successive $\phi^{j*}$s by discrete convolution.

A relevant comment for those attempting to reproduce our results is that, because the normalization employed in (8) is slightly different than the one in the paper, the appropriate kernels $g_k$ for the computation of the image observation $\tilde{d}_\mathrm{obs}$ will not include the normalizing factor $1/\sqrt{\Delta_k}$ that appears in [1]. The reason for the normalization employed here was to preserve the meaning of the approximation in (8) as a density.

### C. Discretization results

The operators that characterize the discretization in [2] are the restriction operators $\mathrm{R}_\mathcal{A}:\mathcal{A}\to\mathcal{A}_{q_1}$ in (9a) and $\mathrm{R}_\mathcal{D}:\mathcal{D}\to\mathcal{D}_{q_2}$ in (9b), and the extensions operators $\mathrm{E}_\mathcal{A}:\mathcal{A}_{q_1}\to\mathcal{A}$ in (10a) and $\mathrm{E}_\mathcal{D}:\mathcal{D}_{q_2}\to\mathcal{D}$ in (10b).

$$\mathrm{R}_\mathcal{A}(a)=\left(\frac{1}{\sqrt{\Delta_k}}\int_{\Lambda_{m,n,k}}a(\mathbf{r},\sigma)\,\mathrm{d}\mathbf{r}\mathrm{d}\sigma\right), \tag{9a}$$

$$\mathrm{R}_\mathcal{D}(d)=\left(\int_{\Lambda_{m,n}}d(\mathbf{r})\,\mathrm{d}\mathbf{r}\right),\forall d\in\mathcal{D}, \tag{9b}$$

$$\mathrm{E}_\mathcal{A}(\tilde{a})=\sum_{n=1}^{N}\sum_{m=1}^{M}\sum_{k=1}^{K}\frac{1}{\sqrt{\Delta_k}}\tilde{a}_{m,n,k}\,i_{\Lambda_{m,n,k}}, \tag{10a}$$

$$\mathrm{E}_\mathcal{D}\left(\tilde{d}\right)=\sum_{n=1}^{N}\sum_{m=1}^{M}\tilde{d}_{m,n}i_{\Lambda_{m,n}}, \tag{10b}$$

These operators allow us to obtain the discrete approximation of the diffusion operator [1, Definition 5] $A:\mathcal{A}\to\mathcal{D}$ in (11a) and its adjoint $A^*\in\mathcal{L}(\mathcal{D},\mathcal{A})$ [1, Lemma 2] in (11b).

$$Aa=\int_0^{\sigma_\mathrm{max}}G_\sigma a_\sigma\mathrm{d}\sigma,\ \forall a\in\mathcal{A}, \tag{11a}$$

$$(A^*d)(\mathbf{r},\sigma)=\mu(\mathbf{r})\cdot\left(G_\sigma\left\{w^2d\right\}\right)(\mathbf{r}),\forall d\in\mathcal{D} \tag{11b}$$

In particular, the finite-dimensional approximations of $A$ and $A^*$ are the operators $\widetilde{A}:\mathcal{A}_{q_1}\to\mathcal{D}_{q_2}$ in (12a) and $\widetilde{A^*}:\mathcal{D}_{q_2}\to\mathcal{A}_{q_1}$ in (12b).

$$\widetilde{A}\tilde{a}=\mathrm{R}_\mathcal{D}\left[A\,\mathrm{E}_\mathcal{A}\left[\tilde{a}\right]\right],\forall\tilde{a}\in\mathcal{A}_{q_1} \tag{12a}$$

$$\widetilde{A^*}\tilde{d}=\mathrm{R}_\mathcal{A}\left[A^*\,\mathrm{E}_\mathcal{D}\left[\tilde{d}\right]\right],\forall\tilde{d}\in\mathcal{D}_{q_2}. \tag{12b}$$

Consider first $\widetilde{A}$. Using (12a) and (10a) we obtain

$$\begin{aligned}\widetilde{A}\tilde{a}&=\mathrm{R}_\mathcal{D}\left[A\,\mathrm{E}_\mathcal{A}\left[\tilde{a}\right]\right]=\mathrm{R}_\mathcal{D}\left[A\sum_{n=1}^{N}\sum_{m=1}^{M}\sum_{k=1}^{K}\frac{1}{\sqrt{\Delta_k}}\tilde{a}_{m,n,k}\,i_{\Lambda_{m,n,k}}\right]=\mathrm{R}_\mathcal{D}\left[\sum_{n=1}^{N}\sum_{m=1}^{M}\sum_{k=1}^{K}\frac{1}{\sqrt{\Delta_k}}\tilde{a}_{m,n,k}Ai_{\Lambda_{m,n,k}}\right]\\&=\mathrm{R}_\mathcal{D}\left[\sum_{n=1}^{N}\sum_{m=1}^{M}\sum_{k=1}^{K}\frac{1}{\sqrt{\Delta_k}}\tilde{a}_{m,n,k}\int_0^{\sigma_\mathrm{max}}G_\sigma i_{\Lambda_{m,n,k}}(\sigma)\mathrm{d}\sigma\right]=\mathrm{R}_\mathcal{D}\left[\sum_{n=1}^{N}\sum_{m=1}^{M}\sum_{k=1}^{K}\frac{1}{\sqrt{\Delta_k}}\tilde{a}_{m,n,k}\int_{\sigma_{k-1}}^{\sigma_k}G_\sigma i_{\Lambda_{m,n}}\mathrm{d}\sigma\right].\end{aligned}$$

Then, using (9b) we obtain

$$\left(\widetilde{A}\tilde{a}\right)_{\tilde{m},\tilde{n}} = \int_{\Lambda_{\tilde{m},\tilde{n}}} \sum_{n=1}^{N} \sum_{m=1}^{M} \sum_{k=1}^{K} \frac{1}{\sqrt{\Delta_k}} \tilde{a}_{m,n,k} \int_{\sigma_{k-1}}^{\sigma_k} G_\sigma i_{\Lambda_{m,n}} \mathrm{d}\sigma \mathrm{d}\mathbf{r}$$
$$= \sum_{k=1}^{K} \sum_{n=1}^{N} \sum_{m=1}^{M} \tilde{a}_{m,n,k} \left( \frac{1}{\sqrt{\Delta_k}} \int_{\sigma_{k-1}}^{\sigma_k} \int_{\Lambda_{\tilde{m},\tilde{n}}} \int_{\Lambda_{m,n}} g_\sigma(\mathbf{r}-\boldsymbol{\rho}) \mathrm{d}\boldsymbol{\rho} \mathrm{d}\mathbf{r} \mathrm{d}\sigma \right) . \quad (13)$$

Consider now $\widetilde{A^*}$. Using (12b) and (10b) we obtain

$$\widetilde{A^*}\tilde{d} = \mathrm{R}_{\mathcal{A}} \left[ A^* \, \mathrm{E}_{\mathcal{D}} \left[ \tilde{d} \right] \right] = \mathrm{R}_{\mathcal{A}} \left[ A^* \sum_{n=1}^{N} \sum_{m=1}^{M} \tilde{d}_{m,n} i_{\Lambda_{m,n}} \right] = \mathrm{R}_{\mathcal{A}} \left[ \sum_{n=1}^{N} \sum_{m=1}^{M} \tilde{d}_{m,n} A^* i_{\Lambda_{m,n}} \right]$$
$$= \mathrm{R}_{\mathcal{A}} \left[ \sum_{n=1}^{N} \sum_{m=1}^{M} \tilde{d}_{m,n} \mu(\mathbf{r}) \left( G_\sigma \left\{ w^2 i_{\Lambda_{m,n}} \right\} \right)(\mathbf{r}) \right] \overset{(!)}{=} \mathrm{R}_{\mathcal{A}} \left[ \sum_{n=1}^{N} \sum_{m=1}^{M} \tilde{d}_{m,n} \tilde{w}_{m,n}^2 \mu(\mathbf{r}) \left( G_\sigma i_{\Lambda_{m,n}} \right)(\mathbf{r}) \right] ,$$

where in (!) we have applied that, because $w$ is a user-provided parameter, it has a discretized structure, i.e. $w = \mathrm{E}_{\mathcal{D}}[\tilde{w}]$. Then, using (9a) we obtain

$$\left(\widetilde{A^*}\tilde{d}\right)_{\tilde{m},\tilde{n},\tilde{k}} = \frac{1}{\sqrt{\Delta_k}} \int_{\Lambda_{\tilde{m},\tilde{n},k}} \sum_{n=1}^{N} \sum_{m=1}^{M} \tilde{d}_{m,n} \tilde{w}_{m,n}^2 \mu(\mathbf{r}) \left( G_\sigma i_{\Lambda_{m,n}} \right)(\mathbf{r}) \mathrm{d}\mathbf{r} \mathrm{d}\sigma$$
$$\overset{(!!)}{=} \tilde{\mu}_{\tilde{m},\tilde{n}} \sum_{n=1}^{N} \sum_{m=1}^{M} \tilde{d}_{m,n} \tilde{w}_{m,n}^2 \frac{1}{\sqrt{\Delta_k}} \int_{\Lambda_{\tilde{m},\tilde{n},k}} \left( G_\sigma i_{\Lambda_{m,n}} \right)(\mathbf{r}) \mathrm{d}\mathbf{r} \mathrm{d}\sigma$$
$$= \tilde{\mu}_{\tilde{m},\tilde{n}} \sum_{n=1}^{N} \sum_{m=1}^{M} \tilde{d}_{m,n} \tilde{w}_{m,n}^2 \left( \frac{1}{\sqrt{\Delta_k}} \int_{\sigma_{k-1}}^{\sigma_k} \int_{\Lambda_{\tilde{m},\tilde{n}}} \left( G_\sigma i_{\Lambda_{m,n}} \right)(\mathbf{r}) \mathrm{d}\mathbf{r} \mathrm{d}\sigma \right)$$
$$= \tilde{\mu}_{\tilde{m},\tilde{n}} \sum_{n=1}^{N} \sum_{m=1}^{M} \tilde{d}_{m,n} \tilde{w}_{m,n}^2 \left( \frac{1}{\sqrt{\Delta_k}} \int_{\sigma_{k-1}}^{\sigma_k} \int_{\Lambda_{\tilde{m},\tilde{n}}} \int_{\Lambda_{m,n}} g_\sigma(\mathbf{r}-\boldsymbol{\rho}) \mathrm{d}\boldsymbol{\rho} \mathrm{d}\mathbf{r} \mathrm{d}\sigma \right) , \quad (14)$$

where in (!!) we have applied that, because $\mu$ is user-provided parameter, it has a discretized structure, i.e. $\mu = \mathrm{E}_{\mathcal{D}}[\tilde{\mu}]$ (note that here we abuse the notation, because in a generic case $\mu \notin \mathcal{D}$. However, the operator $\mathrm{E}_{\mathcal{D}}$ is applicable to $\tilde{\mu} \in \mathbb{T}(M,N)$, and does yield a $\mu \in \mathcal{D}$. This exposes the fact that by restricting $\mu$ to its discretized form we are limiting its support to that represented by our discretization of $\mathcal{D}$.

Let us now analyze the term present both in (13) and (14), i.e.

$$\frac{1}{\sqrt{\Delta_k}} \int_{\sigma_{k-1}}^{\sigma_k} \int_{\Lambda_{\tilde{m},\tilde{n}}} \int_{\Lambda_{m,n}} g_\sigma(\mathbf{r}-\boldsymbol{\rho}) \mathrm{d}\boldsymbol{\rho} \mathrm{d}\mathbf{r} \mathrm{d}\sigma = \frac{1}{\sqrt{\Delta_k}} \int_{\sigma_{k-1}}^{\sigma_k} \int_{\Lambda_{0,0}} \int_{\Lambda_{0,0}} g_\sigma\left( [\tilde{m},\tilde{n}] + \mathbf{r} - [m,n] - \boldsymbol{\rho} \right) \mathrm{d}\boldsymbol{\rho} \mathrm{d}\mathbf{r} \mathrm{d}\sigma$$
$$= \frac{1}{\sqrt{\Delta_k}} \int_{\sigma_{k-1}}^{\sigma_k} \int_{\Lambda_{0,0}} \int_{\Lambda_{0,0}} g_\sigma\left( [\tilde{m}-m, \tilde{n}-n] + \mathbf{r} - \boldsymbol{\rho} \right) \mathrm{d}\boldsymbol{\rho} \mathrm{d}\mathbf{r} \mathrm{d}\sigma \, .$$

Defining $\tilde{g}_k : \mathbb{Z}^2 \to \mathbb{R}_+$ such that

$$\tilde{g}_k[\tilde{\mathbf{r}}] = \frac{1}{\sqrt{\Delta_k}} \int_{\sigma_{k-1}}^{\sigma_k} \int_{\Lambda_{0,0}^2} g_\sigma\left( \tilde{\mathbf{r}} + \boldsymbol{\rho}_1 - \boldsymbol{\rho}_2 \right) \mathrm{d}\boldsymbol{\rho}_1 \times \mathrm{d}\boldsymbol{\rho}_2 \mathrm{d}\sigma, \forall \tilde{\mathbf{r}} \in \mathbb{Z}^2$$

we obtain that for any $\tilde{\alpha} \in \mathbb{T}(M,N)$, if we consider its zero-padded extension $\mathrm{ZP}(\tilde{\alpha}) \in \ell^2$,

$$\sum_{n=1}^{N} \sum_{m=1}^{M} \tilde{\alpha}_{m,n} \tilde{g}_k[(\tilde{m}-m, \tilde{n}-n)] = \sum_{n=-\infty}^{+\infty} \sum_{m=-\infty}^{+\infty} \mathrm{ZP}(\tilde{\alpha})_{m,n} \tilde{g}_k[(\tilde{m}-m, \tilde{n}-n)]$$
$$= \left( g_k * \mathrm{ZP}(\tilde{\alpha}) \right)_{\tilde{m},\tilde{n}} = \left( g_k \circledast \tilde{\alpha} \right)_{\tilde{m},\tilde{n}} ,$$

where $*$ represents discrete convolution and $\circledast$ represents discrete zero-padded convolution. Using this newly introduced discrete convolutional kernels $g_k$ for $k \in \{1, 2, \ldots, K\}$ and the expressions in (13) and (14), then, we directly obtain the discretized operators from [1].

Consider now for a given $\mathbf{r} \in \mathbb{R}^2$, the functional $\vartheta_{\mathbf{r}} : \mathcal{A} \to \mathbb{R}_+$ such that

$$\vartheta_{\mathbf{r}}(a) = \|a_{\mathbf{r},\aleph}\|_{\mathrm{L}^2(\aleph)} = \|\xi a_{\mathbf{r}}\|_{\mathrm{L}^2([0,\sigma_{\max}])} ,$$

with $\xi = 1$ a.e. in $\aleph$ and $0$ a.e. in $\aleph^{\mathrm{c}}$. Let $\mathbf{r} \in \Lambda_{\tilde{m},\tilde{n}}$ for some $(\tilde{n},\tilde{m}) \in \{1,2,\ldots,M\} \times \{1,2,\ldots,N\}$. Then, under the discretization at hand we have that $\vartheta_{\mathbf{r}}$ is approximated by $\tilde{\vartheta}_{\mathbf{r}} : \mathcal{A}_{q_1} \to \mathbb{R}_+$

$$\begin{aligned}\tilde{\vartheta}_{\mathbf{r}}(\tilde{a}) &= \vartheta_{\mathbf{r}}(\mathrm{E}_{\mathcal{A}}[\tilde{a}]) = \vartheta_{\mathbf{r}}\left(\sum_{n=1}^{N}\sum_{m=1}^{M}\sum_{k=1}^{K}\frac{1}{\sqrt{\Delta_k}}\tilde{a}_{m,n,k}\, i_{\Lambda_{m,n,k}}\right) = \left\|\xi\sum_{k=1}^{K}\frac{1}{\sqrt{\Delta_k}}\tilde{a}_{\tilde{m},\tilde{n},k}\, i_{\Lambda_{m,n,k}}\right\|_{\mathrm{L}^2([0,\sigma_{\max}])}\\ &= \sqrt{\int_{\aleph}\left(\sum_{k=1}^{K}\frac{1}{\sqrt{\Delta_k}}\tilde{a}_{\tilde{m},\tilde{n},k}\, i_{\Lambda_{m,n,k}}\right)^2 \mathrm{d}\sigma} = \sqrt{\sum_{k\in\tilde{\aleph}}\int_{\aleph}\frac{1}{\Delta_k}\tilde{a}^2_{\tilde{m},\tilde{n},k}\, i_{\Lambda_{m,n,k}}\mathrm{d}\sigma} = \sqrt{\sum_{k\in\tilde{\aleph}}\tilde{a}^2_{\tilde{m},\tilde{n},k}\frac{1}{\Delta_k}\int_{\aleph} i_{\Lambda_{m,n,k}}\mathrm{d}\sigma}\\ &= \sqrt{\sum_{k\in\tilde{\aleph}}\tilde{a}^2_{\tilde{m},\tilde{n},k}}\,.\end{aligned}$$

## II. Part II – Proximal Optimization and Performance Evaluation

### A. Proximal operator of the non-negative weighted norm in $\mathcal{X}$

In [2, Appendix], we provide the proof of [2, Theorems 1 and 2]. This fundamentally relies on obtaining the proximal operator of the non-negative weighted norm in $\mathcal{X} = \mathrm{L}^2(\aleph)$ with some $\aleph \subset [0,\sigma_{\max}]$. Here, we include Fig. 2 that shows the parallelism between the usual derivation of the prox of a norm and our proof of this result.

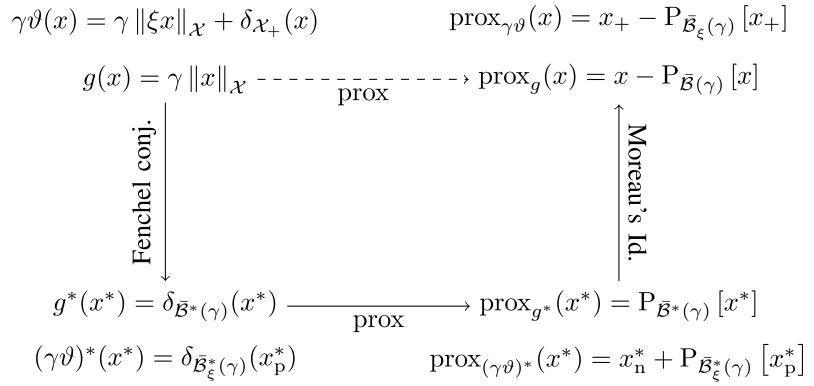


Fig. 2. Schemed followed in [2, Appendix] to show the proximal operator of the non-negative weighted norm in $\mathcal{X}$.

### B. More on kernels and their approximation

Recall here the expression for the discretized kernels obtained in [1], i.e.,

$$\tilde{g}_k[(m,n)] = \frac{1}{\sqrt{\Delta_k}}\int_{\tilde{\sigma}_{k-1}}^{\tilde{\sigma}_k}\omega_{\tilde{\sigma}}(m)\omega_{\tilde{\sigma}}(n)\mathrm{d}\tilde{\sigma} \text{ with } \omega_{\tilde{\sigma}}(m) = \int_{-\frac{1}{2}}^{\frac{1}{2}}\left[\Phi\left(\frac{m+\rho+\frac{1}{2}}{\tilde{\sigma}}\right) - \Phi\left(\frac{m+\rho-\frac{1}{2}}{\tilde{\sigma}}\right)\right]\mathrm{d}\rho\,, \tag{15}$$

and $\Phi : \mathbb{R} \to [0,1]$ is the standard 1D normal cumulative density function. A relevant tip here is that $\omega_{\tilde{\sigma}}(m)$ can be equivalently expressed as

$$\omega_{\tilde{\sigma}}(m) = (m+1)\Phi\left(\frac{m+1}{\tilde{\sigma}}\right) + (m-1)\Phi\left(\frac{m-1}{\tilde{\sigma}}\right) - 2m\Phi\left(\frac{m}{\tilde{\sigma}}\right) + \sigma^2\left[\phi\left(\frac{m+1}{\tilde{\sigma}}\right) + \phi\left(\frac{m-1}{\tilde{\sigma}}\right) - 2\phi\left(\frac{m}{\tilde{\sigma}}\right)\right]. \tag{16}$$

We now introduce two more kernel approximations beside the ones discussed in [2]. The first,

$$g_k^{\mathrm{2ig}}[(m,n)] = \sqrt{\Delta_k}\omega_{\bar{\sigma}_k}(m)\omega_{\bar{\sigma}_k}(m), \text{ where } \bar{\sigma}_k = \tilde{\sigma}_{k-1} + \Delta_k/2,$$

is based on the approximation of the product inside the integral in (15) as a step-constant function in $\tilde{\sigma}$. The second, $g_k^{\mathrm{g}}[\tilde{\mathbf{r}}] = \sqrt{\Delta_k}g_{\bar{\sigma}_k}(\tilde{\mathbf{r}})$, also approximates the spatial integrals involved in obtaining $g_k$, and is convenient for fast implementation and prototyping because libraries for GPU-accelerated Gaussian filtering are readily available on many different platforms. In the next section, one can see that the F1-score differences between the two other approximations, $g_k^{\mathrm{2ig}}$ and $g_k^{\mathrm{g}}$, are not significant. To the authors' surprise, in fact, the performance of the simplest of the approximations, $g_k^{\mathrm{g}}$, seems to be consistently above that of $g_k^{\mathrm{2ig}}$, although not significantly.

## C. Experimental results

The experimental results presented in [2] were selected to be representative, but they did not cover all the scenarios we tested under the same simulation conditions. Figures 3, 4, 5 and 6 include much more information. Parallels to Figures 5 and 6 could be generated for any pair of regularization parameters $\lambda$ and $\lambda_d$ seen in other figures. Furthermore, Figures 7 and 8 are reproductions of figures shown in the paper, but at a larger scale. Here, we first clarify the color coding for all figures reporting F1-Scores.

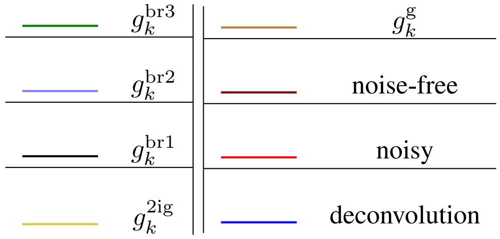


## References

[1] P. del Aguila Pla and J. Jaldén, “Cell detection by functional inverse diffusion and group sparsity – Part I: Modeling and Inverse problems,” *IEEE Transactions on Signal Processing*, 2018, available at: arXiv:1710.01604.

[2] ——, “Cell detection by functional inverse diffusion and group sparsity – Part II: Proximal optimization and Performance evaluation,” *IEEE Transactions on Signal Processing*, 2018, available at: arXiv:1710.01622.

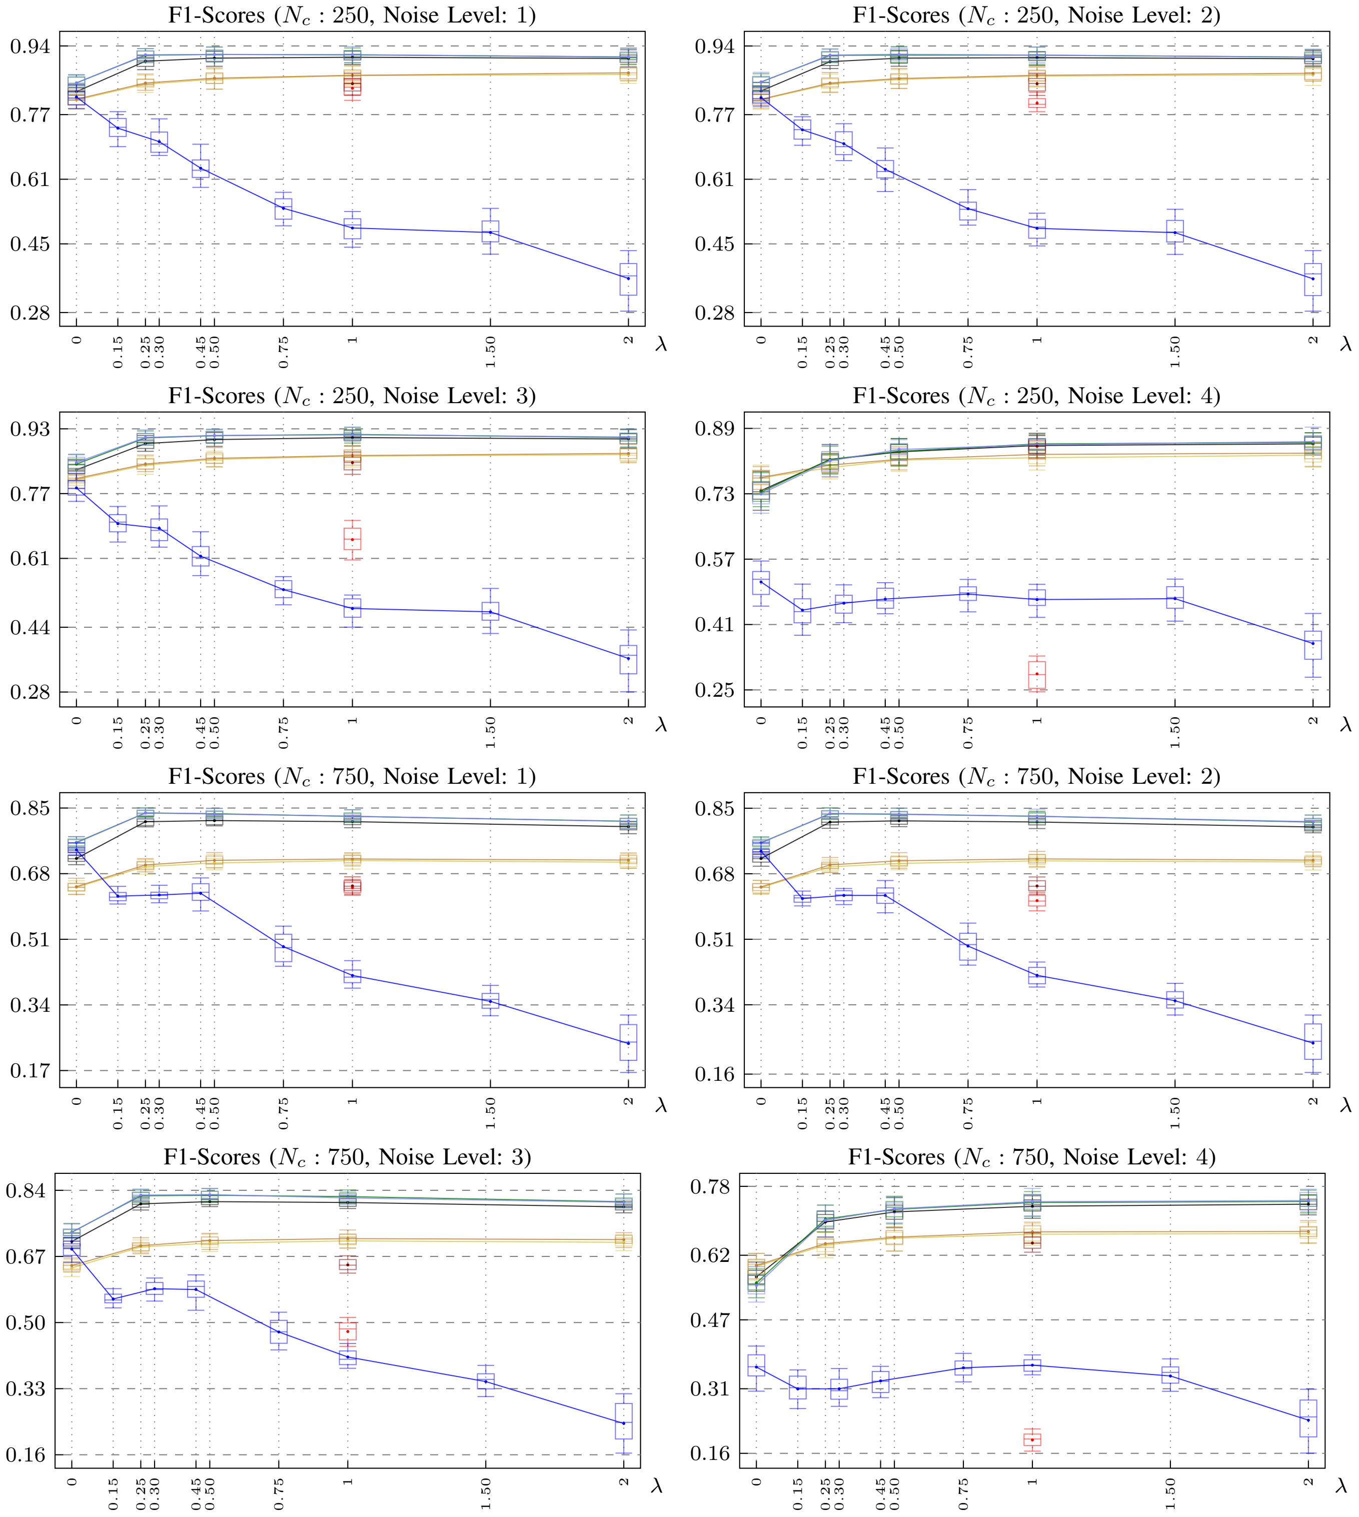


Fig. 3. Statistics of the obtained F1-scores for different methods to obtain $\tilde{p}$. Dependence on the regularization parameter $\lambda$. Those methods that do not use a regularization parameter appear centered in the figure. For parameters and experimental conditons see [2]. For each quantity, a dot and the line illustrate mean behavior, whiskers indicate the evolution of the 10th and 90th percentiles, and the box indicates the evolution of the 25th, 50th and 75th percentiles.

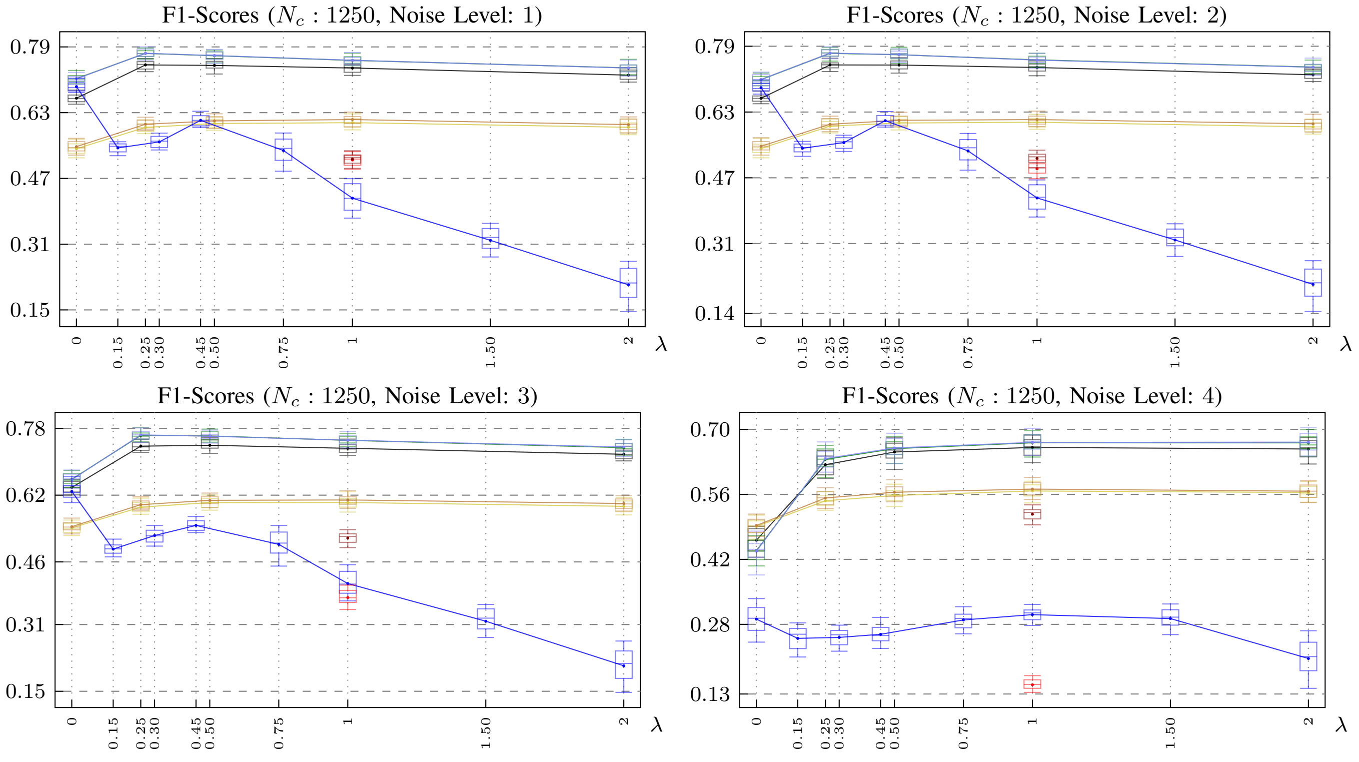


Fig. 4. Statistics of the obtained F1-scores for different methods to obtain $\tilde{p}$. Dependence on the regularization parameter $\lambda$. Those methods that do not use a regularization parameter appear centered in the figure. Color coding as above and reporting of statistics consistent with Figure 3.

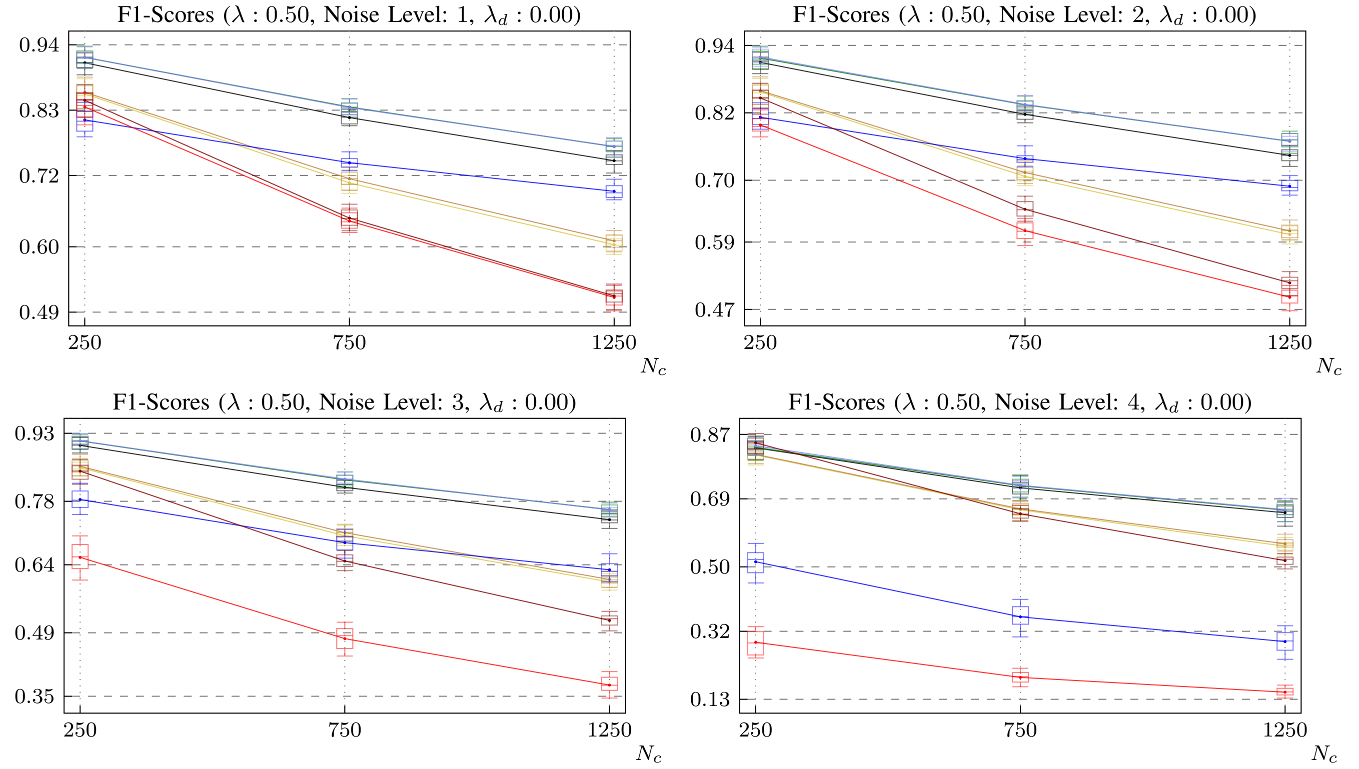


Fig. 5. Statistics of the obtained F1-scores for different methods to obtain $\tilde{p}$. Dependence on the number of active cells in a simulated image $N_c$. Color coding as above and reporting of statistics consistent with Figure 3.

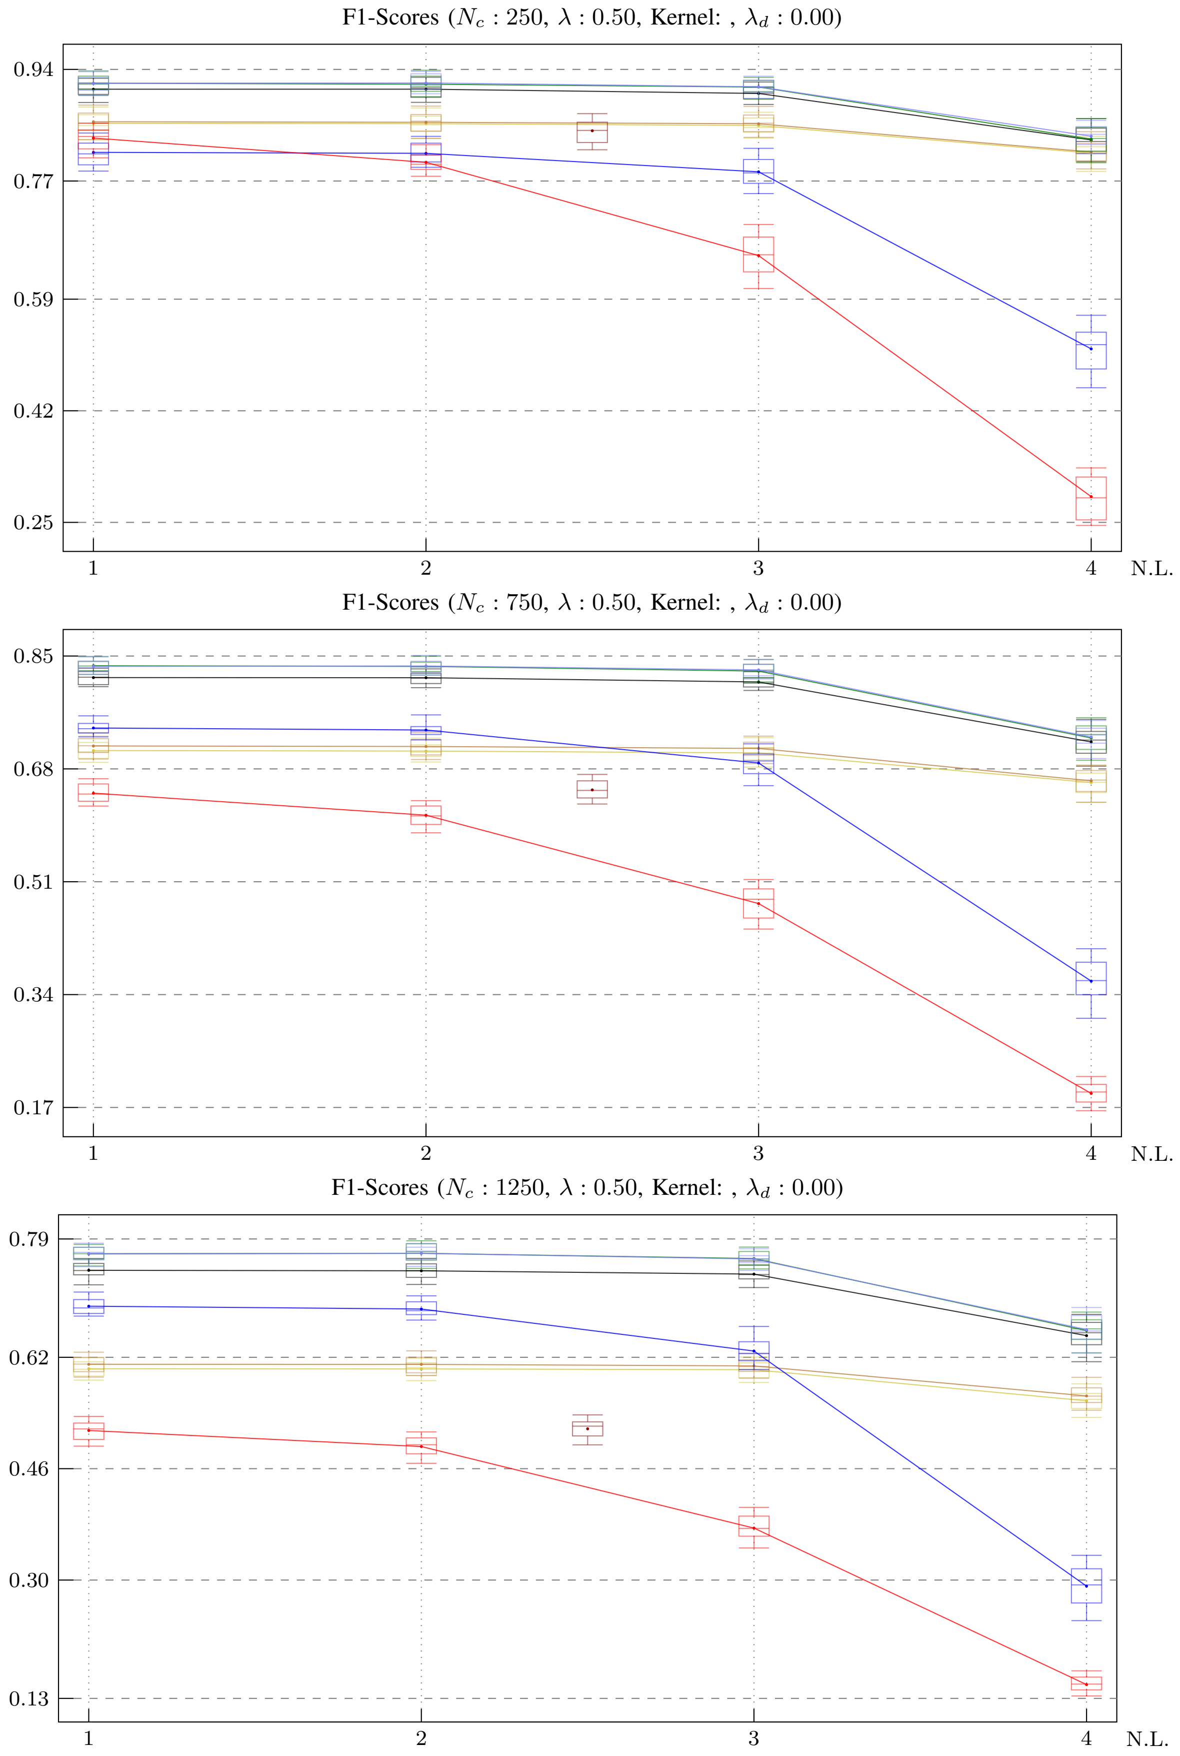


Fig. 6. Statistics of the obtained F1-scores for different methods to obtain $\tilde{p}$. Dependence on the noise level. Color coding as above and reporting of statistics consistent with Figure 3.

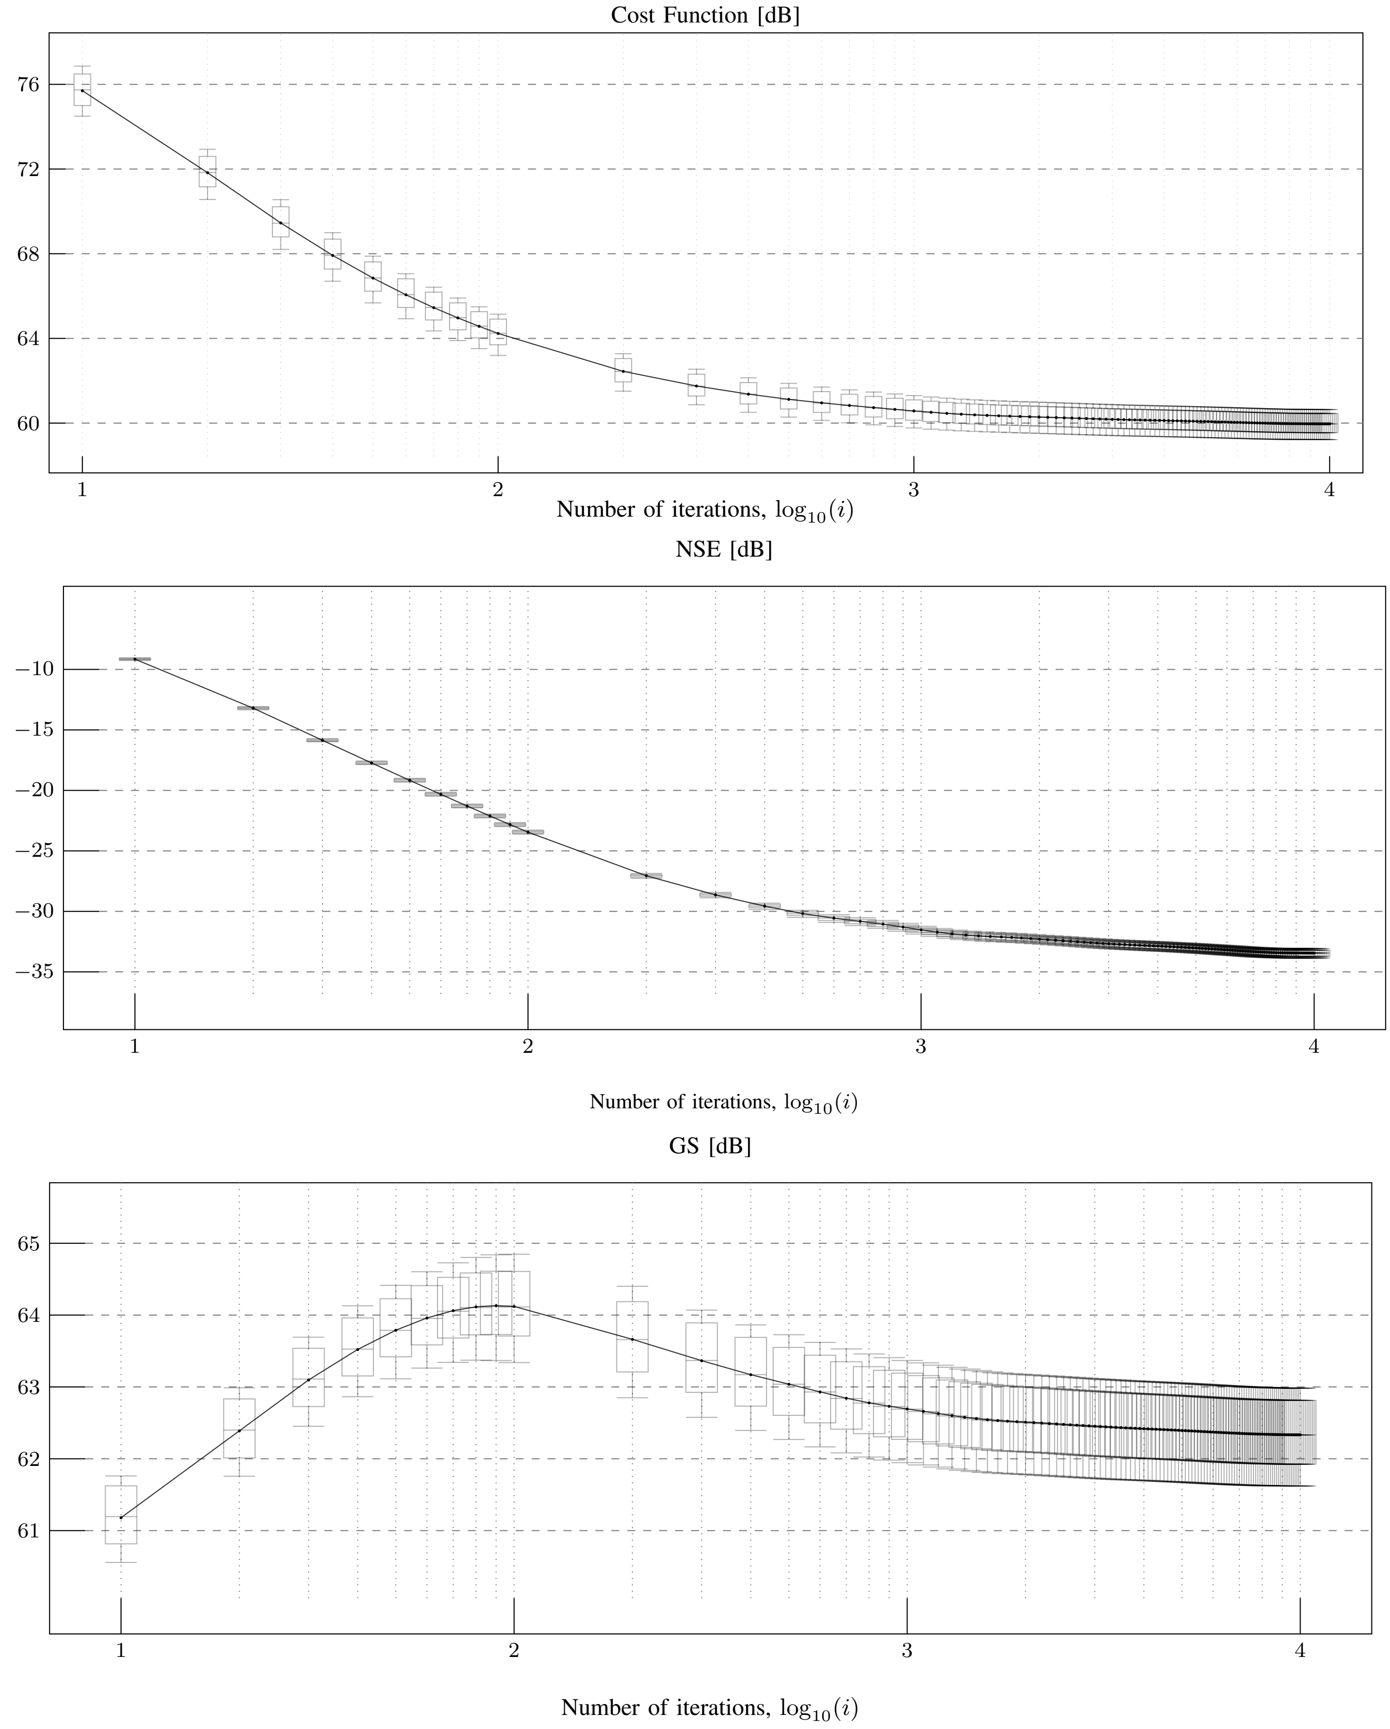


Fig. 7. Statistics of the optimization metrics' evolution. Showing the normalized prediction's square error $\mathrm{NSE} = \|Aa - d_{\mathrm{obs}}\|^2_{\mathcal{D}} / \|d_{\mathrm{obs}}\|^2_{\mathcal{D}}$, the value of the group sparsity regularizer (GS), and the value of the cost function. Comprising results from 50 images with $N_{\mathrm{c}} = 750$ cells and noise level 3 when analyzed with our algorithm with the parameters discussed in the paper and $\lambda = 0.5$. Reporting of statistics consistent with Figure 3. This figure is a larger version of one included in [2].

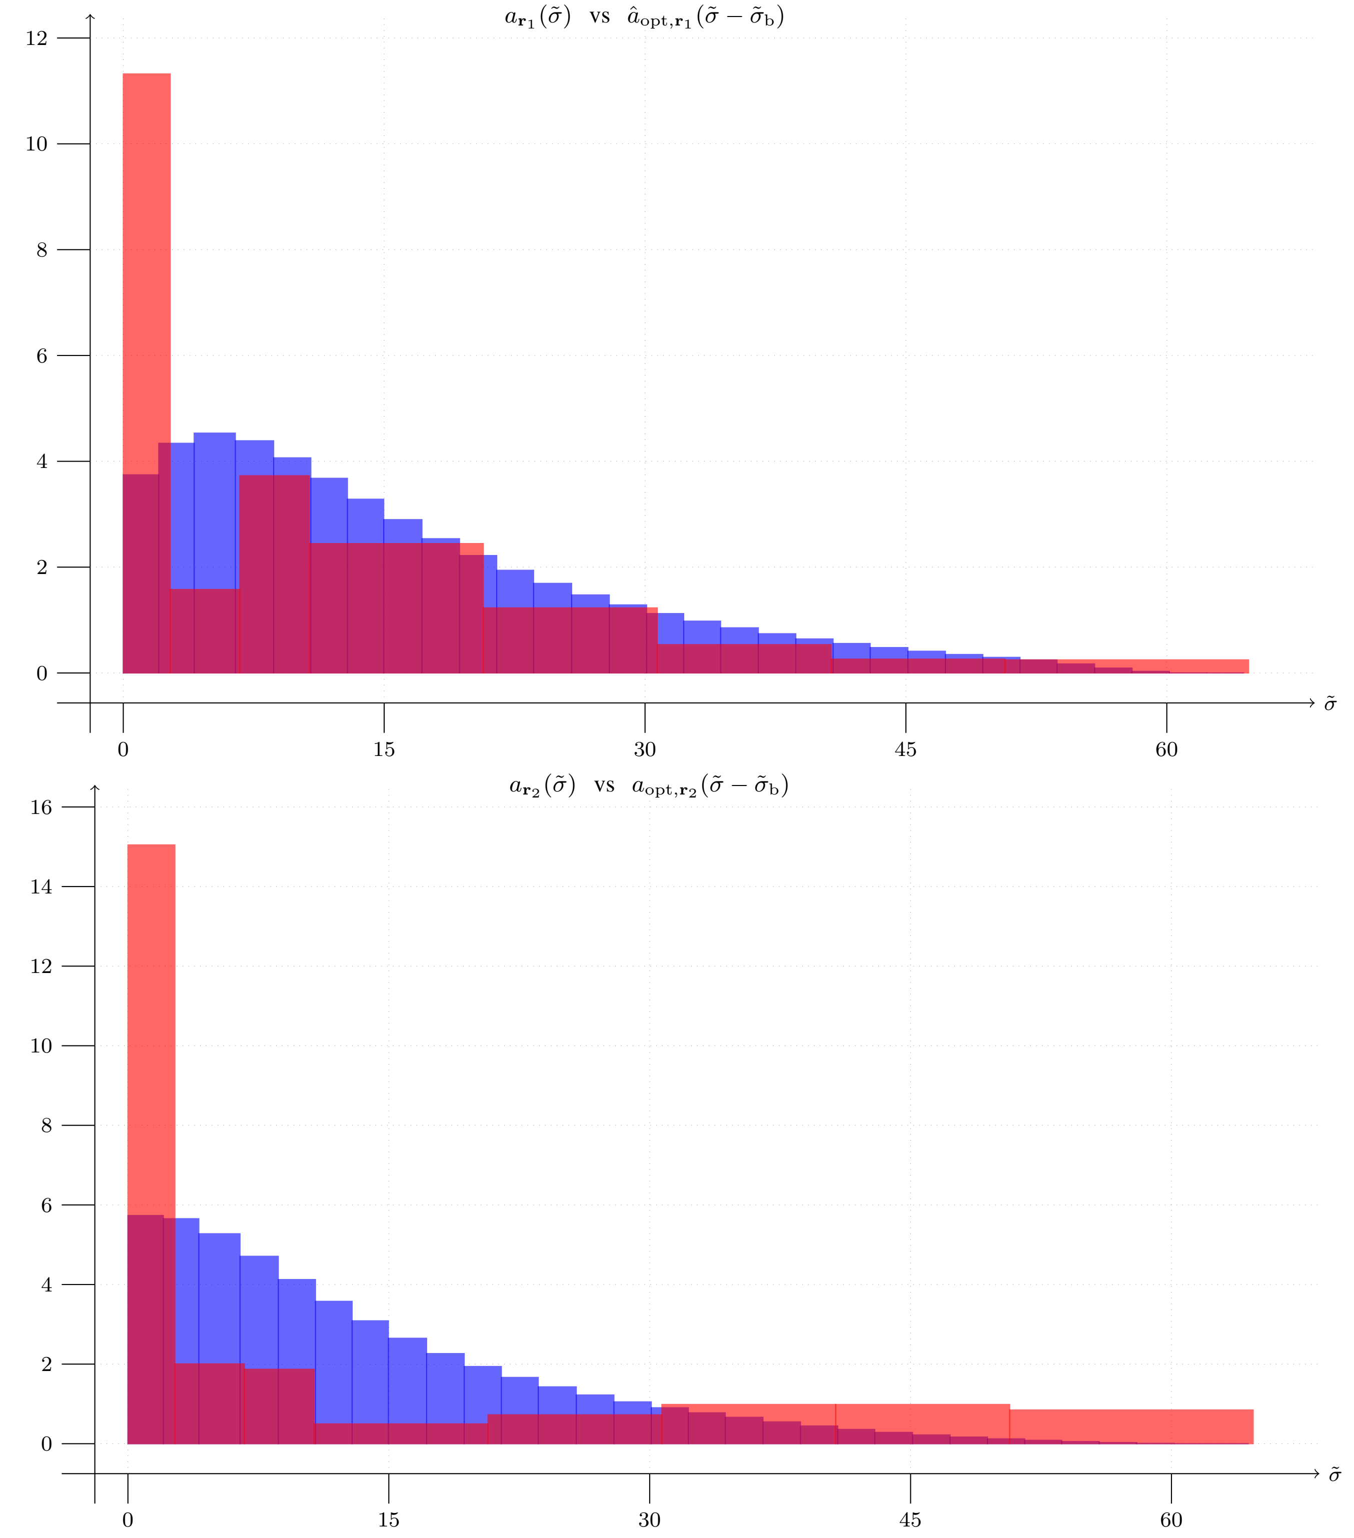


Fig. 8. Two extreme examples of the recovery of $a_{\mathbf{r}}(\tilde{\sigma})$ in simulated spots in different simulation conditions. In blue, $a_{\mathbf{r}}(\tilde{\sigma})$ used to simulate the particular spot, with generation parameters as in the paper. In red, $a_{\mathbf{r}}(\tilde{\sigma})$ recovered by our algorithm with the parameters in the paper, $\lambda = 0.5$, and using the kernel approximations $g_k^{\mathrm{br1}}$. Above, recovery for a cell in an image with $N_{\mathrm{c}} = 1$ and noise level 1. Below, recovery for a well-detected cell in an image with $N_{\mathrm{c}} = 1250$ and noise level 4. The two profiles were normalized to integrate to the same total secretion. This figure is a larger version of on included in [2].
